# Supplementary material for: Typical equilibrium state of an embedded quantum system
Source: arXiv:1707.01820 source file (2017-09-22)
Supplement: Supplementary file 1 [file SuppMat.pdf]

# SUPPLEMENTAL MATERIAL TO TYPICAL EQUILIBRIUM STATE OF AN EMBEDDED QUANTUM SYSTEM

## A. Local Density of States (LDOS)

### *1. Possible shapes for the LDOS*

We review here the various cases for which an expression for the function $f$ in Eq.(4) (i.e. $\mathbb{E}[|\langle\phi_i|\psi_i\rangle|^2]$) is available. For $\hat{H}_0$ with equal energy spacing and $\hat{W}$ in the WBRM ensemble, this function $f$ is predicted to be either a Lorentzian[1–3] with $\Gamma = \pi\sigma_w^2\rho_{s+e}/N$ or an exponential decay[4] with $\Gamma = b/\rho_{s+e}$, depending on whether the band is wide ($b \gg \pi\sigma^2\rho_{s+e}^2/N \gg 1$) or narrow ($1 \ll b \ll \pi\sigma^2\rho_{s+e}^2/N$) respectively. In the former case, the Lorentzian is reminicent of the Breit-Wigner distribution appearing in the deterministic model explaining the capture of slow neutrons by heavy nuclei[5]. The LDOS was also numerically investigated in small Hubbard lattices and found to be Lorentzian[6]. Then, for $\hat{H}_0$ *arbitrary* and $\hat{W}$ belonging to the GOE ensemble, the same Lorentzian shape for $f$ was postulated in the context of thermalisation[7] and recently established in the context of financial data analysis [8, 9] also in the non perturbative case. In addition, *free* probability tools[10–12] provide an extension of this Lorentzian to the case $\hat{H}_0$ arbitrary and $\hat{W}$ in the RRM ensembles: the energy scale $\Gamma = \pi\sigma_w^2\rho_{s+e}/N$ can then be seen as a truncation at second order of an expansion over the *free* cumulants of the interaction. Finally, we can mention that the LDOS was considered for $W$ in an *embedded* ensemble, the Two Body Random Interaction (TBRI) ensemble which is refinement of WBRM enforcing a two body nature of the interaction, and which is relevant in the context of heavy nuclei[13] and atoms, atomic clusters and quantum dots. A crossover from a Lorentzian to a gaussian behavior is numerically observed and predicted (see for instance [14, 15] and the review in[16]). It is important to stress here that a Lorentzian (or Breit-Wigner) distribution for the LDOS and consequently for $\bar{p}_{m\to n}$ does *not* preclude thermalisation as far as the state of the subsystem $S$ is concerned, as we will explain now.

### *2. Discussion on the shape of the LDOS and the conditions for thermalisation*

There is numerical evidence that a Gaussian LDOS (or strength function SF) is necessary for the onset of thermalisation in systems of interacting particles[17–19], as far as observables of these closed systems are concerned. To summarize the conclusion of the review article[19]: one prerequisite for thermalization in closed quantum systems made of interacting particles is the equivalence between the width of the strength function and the width of the energy shell. In other words, an initial bare state should be completely delocalized over the dressed eigenvectors. This is the so called chaotic eigenstates configuration, whose emergence in systems made of interacting particles is associated with the crossover of the strength function from a Breit-Wigner to a Gaussian law. Such configuration is required for thermalization because the initial state is then a large superposition of many components (the chaotic eigenstates) and expectation values of observables (e.g. particle number) on this state are large sums of uncorrelated or weakly correlated terms (See, e.g., Eqs.(5.4) (5.5) and (7.1) in [19]). As a consequence, these sums are the subject of a generalized central limit theorem: they are *self-averaging*, making them independent of microscopic details and smooth functions of the total energy. Such insensitivity of expectation values of observables to microscopic details is clearly the first property one should expect from a statistical description of the system under consideration. This is why, in these systems, the emergence of chaotic eigenstates filling the energy shell and the associated crossover of the SF from Breit-Wigner to Gaussian is required for the onset of thermalization. It is important to stress that this property concerns observables defined on the total Hilbert space of a closed quantum system made of interacting particles.

When on considers the state of a system coupled to a large environment, as we do here, the situation is different. Indeed, in this case, because of dynamical typicality[20], the reduced density matrix of S (i.e. the state of S) is self-averaging (or typical) whatever the level of delocalization of the initial bare state in the dressed eigenbasis. The only condition for typicality is a large dimension for the Hilbert space of the environment. This means that a statistical description of the system is possible even if the Strength Function follows a Breit-Wigner law.

In other words, the transition probability defined on the full composite system: $p_{m\to n}$ from Eq.(3) might not be self averaging (if the SF does not fill the energy shell, e.g. with a Breit-Wigner distribution), but the state of S obtained from this quantity after partial tracing *is* self averaging provided $\dim(\mathcal{H}_e)$ is large. As a consequence, the state of $S$ does not depend on microscopic details and a statistical description is possible, which is the prerequisite for thermalization.

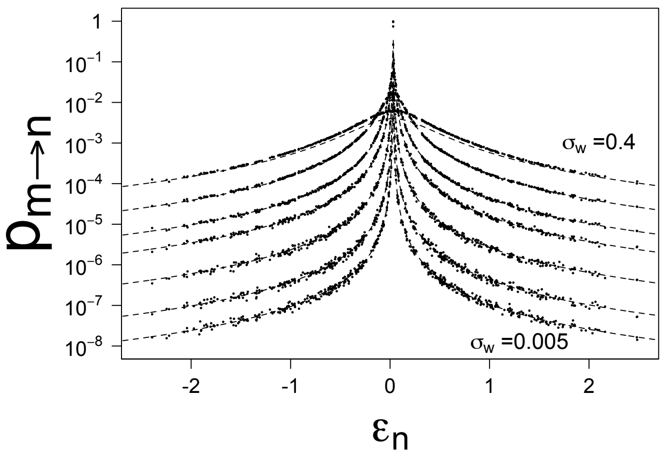


FIG. 1. **Average transition probability $\bar{p}_{m\to n}$ from an initial bare state $|\phi_m\rangle$ at $t = 0$ to a final bare state $|\phi_n\rangle$ at $t \to \infty$.** The bare Hamiltonian $\hat{H}_0$ is chosen with a gaussian density of states and $\hat{W}$ is in the GOE. The initial state $|\phi_m\rangle$ is chosen to be in the center of the spectrum $\epsilon_m \approx 0$ . $\bar{p}_{m\to n}$ is plotted as a function of $\epsilon_n$ and for different interaction strengths ($\sigma_w = 0.005, 0.01, 0.025, 0.06, 0.1, 0.2, 0.4$). This average transition probability quantifies how other bare states are *accessible* from $|\phi_m\rangle$. The theoretical prediction (dashed line) is provided by Eq.(5) (main body of the article) with $g(\epsilon) = \frac{\sigma_w^2}{N}\frac{2}{\epsilon^2+4\Gamma^2}$ and $\Gamma = \pi^2\sigma_w^2\rho/N$ and has universal properties: it only depends on the local behavior of the density of states of the dressed Hamiltonian $\rho$ and the typical strength of the interaction $\sigma_w$. In addition, it has a Lorentzian shape, in sharp contrast to equiprobability.

Finally, one should also note that the main analytical result in Eq.(6) is checked numerically in the Fig.1 of the main body of the article on the simple example of a two level system coupled to a environment through an interaction in the GOE ensemble. In the intermediate regime where the strength function follows a Breit-Wigner law, the system S can be clearly seen to thermalize and the agreement with the theoretical prediction is satisfactory.

## B. Numerical simulations

### *1. Average transition probability between bare states: $\bar{p}_{m\to n}$.*

We consider here numerically the transition probability $p_{m\to n}$ between two bare states (i.e. eigenvectors of $\hat{H}_0 = \hat{H}_e + \hat{H}_s$): $|\phi_m\rangle$ at $t = 0$ and $|\phi_n\rangle$ at $t \to \infty$ (see Fig.1) The total Hilbert space dimension is set to $N = 500$, the density of states of $\hat{H}_0$ is chosen to be centered and Gaussian distributed with variance $\sigma_0^2 = \mathrm{Tr}(\hat{H}_0^2)/N = 1$. The interaction $\hat{W}$ is a real symmetric matrix such that $\{W_{i,j}\}_{i\geqslant j}$ are independent identically distributed centered Gaussians with standard deviation $\sigma_w/\sqrt{N}$ (providing $\mathrm{Tr}(\hat{W}^2)/N = \sigma_w^2$). Diagonalizing numerically the dressed Hamiltonian $\hat{H}_0 + \hat{W}$ provides the overlap or transfer matrix of general term $\langle\psi_i|\phi_n\rangle$. The empirical average of $p_{m\to n} = \sum_i |\langle\phi_n|\psi_i\rangle|^2|\langle\phi_m|\psi_i\rangle|^2$ is computed over 100 realization of $\hat{W}$, for a fixed value of the initial energy ($\epsilon_m \approx 0$, i.e. middle of the spectrum) and as a function of $\epsilon_n$ for different interaction strengths $\sigma_w$.

### *2. Cross over between a local microcanonical ensemble and a global microcanonical ensemble. Details for Fig.1 of the main body of the article*

We consider here numerically the particular case of a two level system $S$ (gap $\Delta = 2$). The density of states of the environment $\rho_e$ is chosen to be Gaussian distributed (standard deviation $\sigma_e = 1$) which is suitable e.g. for small Hubbard lattices[6]. We take the interaction $\hat{W}$ in the GOE ensemble: written in the eigenbasis of $\hat{H}_s + \hat{H}_e$, the interaction $\hat{W}$ is real symmetric such that $\{W_{i,j}\}_{i\geqslant j}$ are independent centered Gaussians with standard deviation $\sigma_w/\sqrt{\dim\mathcal{H}}$ (providing $\mathrm{Tr}(\hat{W}^2)/\dim\mathcal{H} = \sigma_w^2$). The environment Hilbert space dimension is set to $\dim\mathcal{H}_e = 4096$, the initial state to

$|1_s\rangle\langle 1_s|\otimes|2048_e\rangle\langle 2048_e|$ (i.e. middle of the spectrum for $E$: $\epsilon_e \approx 0$) and we numerically integrate the Schrödinger equation for different values of the interaction strength $\sigma_w = \sqrt{\mathrm{Tr}(W^2)/N} = 0.2, 0.4, 0.5, 0.7, 0.91, 1.11, 1.41, 2.0, 3.0, 9.1$. We calculate the reduced density matrix of $S$ from which we extract one diagonal component: the probability $P_1$. After a transient regime at short times ($t \lesssim 4$), a stationary regime takes place. We extract the time average of $P_1$ and plot it as a function of the interaction strength on the right panel (points). As the interaction strength increases, the time average value of $P_1$ goes from a *local* micro-canonical prediction $P_1 \approx \rho_e(\Delta)/(\rho_e(\Delta)+\rho_e(0)) \approx 0.87$ to a *global* microcanonical prediction: $P_1 \approx 0.5$. The analytical prediction for this crossover (in dash) is given by Eq.(6) which can be calculated analytically when $\rho_e$ is gaussian and $g$ a Lorentzian: $V(\Delta, \sigma_{e+s}, \Gamma')/(V(\Delta, \sigma_{e+s}, \Gamma')+V(0, \sigma_{e+s}, \Gamma'))$ where $V(\epsilon, \sigma_{s+e}, \Gamma')$ is the Voigt function[21], i.e. the convolution of a Gaussian (standard deviation $\sigma_{e+s}$) with a Lorentzian (width $\Gamma'$). We use $\sigma_{e+s}^2 = \sigma_e^2 + \sigma_s^2 = 2$ and $\Gamma' = 2\pi\sigma_w^2\rho/N$ where $\rho$ is the *dressed* density of states. It is crucial here to take into account the dependence of $\rho$ on the interaction strength. For this purpose, we make the crude approximation of considering $\hat{H}_0$ and $\hat{W}$ like two GOE random matrices, so that the spectrum of $\hat{H}_0 + \hat{W}$ is a semi circle law $\rho(\lambda) = \frac{N\pi}{2R^2}\sqrt{R^2-\lambda^2}$ whose variance $\sigma^2 = R^2/4$ is the sum of the spectral variances of $\hat{H}_0$ and $\hat{W}$[22]: $\sigma^2 = \sigma_{e+s}^2 + \sigma_w^2$ and $\lambda \approx \Delta$ is the initial energy.

### C. Fourth order statistics of the overlap coefficients $\mathbb{E}[\langle\phi_n|\psi_i\rangle\langle\psi_i\phi_m\rangle\langle\phi_p|\psi_j\rangle\langle\psi_j|\phi_q\rangle]$: zero cases

The purpose of this section is to spot the cases for which the quantity $\mathbb{E}[\langle\phi_n|\psi_i\rangle\langle\psi_i\phi_m\rangle\langle\phi_p|\psi_j\rangle\langle\psi_j|\phi_q\rangle]$ is zero. For this purpose, we use the well known fact that the overlap product $\langle\phi_n|\psi_i\rangle\langle\psi_i|\phi_m\rangle$ is (up to a factor $2\pi$) the residue of the matrix element of the resolvent operator $G_H(z) = (H - z\mathbb{1})^{-1}$ at the pole $\lambda_i$ since the expansion in the dressed basis provides $G_{n,m}(z) = \langle\phi_n|G_H(z)|\phi_m\rangle = \sum_i \langle\phi_n|\psi_i\rangle\langle\psi_i|\phi_m\rangle/(\lambda_i - z)$. We are thus lead to consider the equivalent problem of finding the cases for which $\mathbb{E}[G_{n,m}(z_1)G_{p,q}(z_2)]$ is zero for all $z_1, z_2$ outside the spectrum of $\hat{H}$.

#### 1. Zero cases for the first and second order statistics of the resolvent entries

The aim of this section is to prove that the only non zero correlations between matrix elements of the resolvent operator $\mathbb{E}[G_{n,m}(z_1)G_{p,q}(z_2)]$ are when ($n = q$ and $m = p$) or ($n = m$ and $p = q$). The first case will contribute to both the transient and the stationary regimes of the *diagonal* terms of the total density matrix, whereas the last case ($n = m$ and $p = q$) provides both regimes of the extra diagonal terms (or quantum coherences) of $\varrho(t)$. In the main part of the paper, we focus on the first case. We provide in Section C an explanation why the second case can be neglected as far as the stationary regime of the subsystem $S$ is concerned.

We will first focus on the case where the interaction is a randomly rotated matrix: i.e. $\hat{W} = \hat{U}.\hat{Q}.\hat{U}^\dagger$ with $\hat{U}$ unitary or orthogonal distributed according to the Haar measure. Then we will explain how a similar reasoning provides the same result in the case where $\hat{W}$ is a Wigner Random Band Matrix with entries having an even probability distribution.

#### 2. Case $\hat{W} = \hat{U}.\hat{Q}.\hat{U}^\dagger$ with $\hat{U}$ unitary or orthogonal, both distributed according to the Haar measure

To proceed, we first remind the results from Kargin [12] on the average of the resolvent operator $G_{\hat{H}}(z) = \frac{1}{\hat{H}-z\mathbb{1}}$, defined for $z \in \mathbb{C}\backslash\mathbb{R}$, where $\hat{H} = \hat{H}_0 + \hat{P}.\hat{Q}.\hat{P}^\dagger$ with $\hat{H}_0$ a $N \times N$ hermitian deterministic matrix, $\hat{P}$ unitary Haar distributed and $\hat{Q}$ real deterministic diagonal. The main result being that this average is actually diagonal in the eigenbasis of $\hat{H}_0$. Then we adapt Kargin's method to get our result on the second order statistics (the correlations between resolvent entries). In the following lemma and its proof, we shall write the matrices in an eigenbasis $\{|\phi_1\rangle, \ldots, |\phi_N\rangle\}$ of $\hat{H}_0$, so that we can suppose that $\hat{H}_0$ is a diagonal matrix. Besides, by invariance of the Haar measure (i.e. by the fact that for any fixed unitary matrix $\hat{O}$, $\hat{P}\hat{O}$ is also distributed according to the Haar measure), one can suppose that $\hat{Q}$ is diagonal.

Let $z, z_1, z_2 \in \mathbb{C}\backslash\mathbb{R}$. We have

(a) The matrix $\mathbb{E}[G_{\hat{H}}(z)]$ is diagonal.

(b) The matrix $\mathbb{E}[G_{\hat{H}}(z_1)\hat{M}G_{\hat{H}}(z_2)]$ is diagonal for any diagonal matrix $\hat{M}$.

(c) For any $i \neq j$, for $\hat{M}_{i,j}$ the matrix whose sole non-zero entry is the $(i,j)$-th one, the only non-zero entry of the matrix $\mathbb{E}[G_{\hat{H}}(z_1)\hat{M}_{i,j}G_{\hat{H}}(z_2)]$ is the $(i,j)$-th one.

*Proof.* Let $p_{ij}$ denote the entries of the unitary matrix $P$ and set $q_{ij} := p_{ji}^*$ (here, $^*$ stands for the complex conjugate). Note that in each proposition, by analytic continuation, it suffices to focus on large enough $z, z_1, z_2$. In this case, using the formula

$$\frac{1}{\hat{H}_0 + \hat{P}.\hat{Q}.\hat{P}^\dagger - z\mathbb{1}} = -\sum_{k\geq 0} \frac{(\hat{H}_0 + \hat{P}.\hat{Q}.\hat{P}^\dagger)^k}{z^{k+1}}$$

(which is true as soon as $|z| > \|\hat{H}_0\| + \|\hat{Q}\|$), the expansion of $\hat{H}_0 + \hat{P}.\hat{Q}.\hat{P}^\dagger$ and the fact that both $\hat{H}_0$ and $\hat{Q}$ are diagonal, the propositions of the lemma reduce to the following ones:

(a') For any $p \geq 0$, any $A_1, \ldots, A_{2p}$ diagonal matrices, the matrix

$$\mathbb{E}[A_1\hat{P}A_2\hat{P}^\dagger \cdots A_{2p-1}\hat{P}A_{2p}\hat{P}^\dagger]$$

is diagonal.

(b') Same as (a').

(c') For any $p, q \geq 0$, any $A_1, \ldots, A_{2p}$, $B_1, \ldots, B_{2q}$ diagonal matrices and any matrix $M_{i,j}$ whose sole non-zero entry if the $(i,j)$-th one (with $i \neq j$), the only non-zero entry of the matrix

$$\mathbb{E}[A_1\hat{P}A_2\hat{P}^\dagger \cdots A_{2p-1}\hat{P}A_{2p}\hat{P}^\dagger M_{ij} B_1\hat{P}B_2\hat{P}^\dagger \cdots B_{2q-1}\hat{P}B_{2q}\hat{P}^\dagger]$$

is the $(i,j)$-th one.

Expanding the matrix products, (a"') and (c"') then reduce to

(a") For any $k \geq 1$, any $i_1, \ldots, i_{k+1}$, $j_1, \ldots, j_k$, we have

$$i_1 \neq i_{k+1} \implies \mathbb{E}[p_{i_1j_1}q_{j_1i_2}p_{i_2j_2}q_{j_2i_3} \cdot \cdots \cdot p_{i_kj_k}q_{j_ki_{k+1}}] = 0.$$

(c") For any $k, l \geq 1$, any $i_1, \ldots, i_{k+1}$, $j_1, \ldots, j_k$, any $a_1, \ldots, a_{l+1}$, $b_1, \ldots, b_l$, such that $i_{k+1} \neq a_1$, we have

$$\mathbb{E}[p_{i_1j_1}q_{j_1i_2} \cdots p_{i_kj_k}q_{j_ki_{k+1}} \times p_{a_1b_1}q_{b_1a_2} \cdots p_{a_lb_l}q_{b_la_{l+1}}] \neq 0$$
$$\implies i_1 = i_{k+1} \text{ and } a_1 = a_{l+1}.$$

It is easy to see that (c") reduces to (a"). So let us prove (a"). By invariance of the Haar measure by left and right multiplication by diagonal matrices with diagonal entries on the unit circle of $\mathbb{C}$, we know that for the above expectation to be non zero, the number of times an index $i$ appears as first coordinate of a $p_{kl}$ term to be equal to the number of times it appears as the second coordinate of a $q_{kl}$ term. This constraint cannot be satisfied if $i_1 \neq i_{p+1}$.

### *3. Case $W$ is a Wigner Random Band Matrix*

The very same reasoning can be applied in the case where $W$ is a Wigner Band Random Matrix. In this case, the crucial hypothesis for obtaining the result is that the distribution of each entry should be even. Propositions (a'),(b'),(c') from the previous section are changed for the following ones:

(a"') For any $p \geq 0$, any $A_1, \ldots, A_p$ diagonal matrices, the matrix

$$\mathbb{E}[A_1WA_2W \cdots A_pW]$$

is diagonal.

(b"') Same as (a"').

(c''') For any $p, q \geq 0$, any $A_1, \ldots, A_p$, $B_1, \ldots, B_q$ diagonal matrices and any matrix $M_{i,j}$ whose sole non-zero entry is the $(i, j)$-th one (with $i \neq j$), the only non-zero entry of the matrix

$$\mathbb{E}[A_1 W \cdots A_p W M_{ij} B_1 W \cdots B_q W]$$

is the $(i, j)$-th one.

Defining $w_{i,j}$ for the $(i, j)$ entry of $\hat{W}$ and expanding the matrix products, (a''') and (c''') then reduce to

(a'''') For any $k \geq 1$, any $i_1, \ldots, i_{k+1}$, we have

$$i_1 \neq i_{k+1} \implies \mathbb{E}[w_{i_1,i_2} w_{i_2,i_3} w_{i_3,i_4} \cdot \cdots \cdot w_{i_k,i_{k+1}}] = 0.$$

(c'''') For any $k, l \geq 1$, any $i_1, \ldots, i_{k+1}$, any $a_1, \ldots, a_{l+1}$, such that $i_{k+1} \neq a_1$, we have

$$\mathbb{E}[w_{i_1,i_2} w_{i_2,i_3} \cdots w_{i_k,i_{k+1}} \times w_{a_1,a_2} w_{a_2,a_3} \cdots w_{a_l a_{l+1}}] \neq 0 \\ \implies i_1 = i_{k+1} \text{ and } a_1 = a_{l+1}.$$

It is easy to see that (c'''') reduces to (a''''). So let us prove (a''''). From the even character of the probability distribution of each entry of $\hat{W}$ and their pairwise statistical independence, we know that, for the above expectation to be non zero, the number of times an index $i$ appears in the product $w_{i_1,i_2}, \ldots$ has to be even. This constraint cannot be satisfied if $i_1 \neq i_{k+1}$.

### D. Stationary regime of the extra diagonal terms of $\varrho(t)$: case ($n = m$ and $p = q$).

In the long time limit, the matrix element $\mathbb{E}[\langle\phi_n|U_t|\phi_n\rangle\langle\phi_p|U_t^\dagger|\phi_p\rangle]$ is equal to the same diagonal sum of residues as considered in the main body of the text: $\sum_i \mathbb{E}[|\langle\phi_n|\psi_i\rangle|^2|\langle\phi_p|\psi_i\rangle|^2]$, however here the partial trace operation imposes a strong constraint on $|\epsilon_n - \epsilon_p|$ to get a non zero contribution to the extra diagonal matrix element of the reduced density matrix of $S$: $|\epsilon_n - \epsilon_p|$ is always larger that $D_s$ the minimum level spacing of the system $S$ alone. As a consequence, the extra diagonal terms of the reduced density matrix of $S$ in the long time limit (i.e. $\lim_{t\to\infty}\langle\epsilon_s|\varrho_s(t)|\epsilon_{s'}\rangle$ for $s \neq s'$) will always be smaller than their diagonal counterparts (i.e. $\lim_{t\to\infty}\langle\epsilon_s|\varrho_s(t)|\epsilon_s\rangle$) by a factor equal to $\Gamma'^2$ (the square of the width of the $\bar{p}_{m\to n}$ curve) over $D_s^2$. In this paper, we will assume $\Gamma' \ll D_s$ as a start but it would be interesting to investigate the other regime.


[1] E. P. Wigner, Annals of Mathematics **62**, 548 (1955).
[2] E. P. Wigner, Annals of Mathematics **65**, 203 (1957).
[3] Y. V. Fyodorov, O. A. Chubykalo, F. M. Izrailev, and G. Casati, Physical Review Letters **76**, 1603 (1996).
[4] V. V. Flambaum, A. A. Gribakina, G. F. Gribakin, and M. G. Kozlov, Physical Review A **50**, 267 (1994).
[5] G. Breit and E. Wigner, Phys. Rev. **49**, 519 (1936).
[6] S. Genway, A. F. Ho, and D. K. K. Lee, Physical Review A **86** (2012).
[7] J. M. Deutsch, Physical Review A **43**, 2046 (1991).
[8] R. Allez and J.-P. Bouchaud, Random Matrices: Theory Appl. **03** (2014).
[9] R. Allez, J. Bun, and J.-P. Bouchaud, arXiv:1412.7108 [cond-mat] (2014), arXiv: 1412.7108.
[10] D. Voiculescu, J. Funct. Anal. **66** (1986).
[11] P. Biane, arXiv e-prints (1998), math/9809193.
[12] V. Kargin, Ann. Probab. **43**, 2119 (2015).
[13] V. V. Flambaum, G. F. Gribakin, and F. M. Izrailev, Physical Review E **53**, 5729 (1996).
[14] V. V. Flambaum, F. M. Izrailev, and G. Casati, Phys. Rev. E **54**, 2136 (1996).
[15] V. Flambaum and F. Izrailev, Physical Review E **61**.
[16] V. K. B. Kota, *Embedded Random Matrix Ensembles in Quantum Physics* (Springer, 2014).
[17] L. F. Santos, F. Borgonovi, and F. M. Izrailev, Physical Review Letters **108**, 094102 (2012).
[18] E. J. Torres-Herrera, M. Vyas, and L. F. Santos, New Journal of Physics **16**, 063010 (2014).
[19] F. Borgonovi, F. M. Izrailev, L. F. Santos, and V. G. Zelevinsky, Physics Reports Quantum chaos and thermalization in isolated systems of interacting particles, **626**, 1 (2016).
[20] G. Ithier and F. Benaych-Georges, Physical Review A **96**, 012108 (2017).
[21] W. Voigt, Munch. Ber. **603** (1912).
[22] O. Z. G. Anderson, A. Guionnet, An Introduction to Random Matrices, Vol. 118 (Cambridge studies in advanced mathematics, 2009).
